# Supplementary material for: Diffusion Probabilistic Models for Structured Node Classification
Source: arXiv:2302.10506 source file (2023-06-19)
Supplement: Supplementary file 1 [file model_architecture.tex]

\section{Detailed descriptions of DPM-GSP}
\label{appx:architecture}

In this section, we describe the detailed components of DPM-GSP. 

\subsection{Variances schedule} \label{appx:architecture_diffusion} To determine the variances schedule $\beta_1,\ldots,\beta_T$, we use the cosine beta schedule suggested by \citep{nichol2021improved}. Here, we set the offset parameter to $0.008$.

\subsection{Detailed reverse diffusion process} \label{appx:architecture_reverse} In \Cref{subsec:method-inductive}, we parameterize probabilistic distribution of the reverse diffusion step $p_{\bm{\theta}}(\bm{y}^{(t-1)}|\bm{y}^{(t)})$ as $\mathcal{N}(\bm{y}^{(t-1)};\bm{\mu}_{\bm{\theta}}(\bm{x},\bm{y}^{(t)},G,t),\sigma_t^2)$. Here, we set $\sigma_t^2$ to $\beta_t$. Following \citep{ho2020denoising}, we also define $\mu_{\bm{\theta}}(\bm{x},\bm{y}^{(t)},G,t)$ as follows:
\begin{align} %\label{eq:epsilon_pred}
\mu_{\bm{\theta}}(\bm{x},\bm{y}^{(t)},G,t)=\frac{1}{\sqrt{\alpha_t}}\left(\bm{y}^{(t)}-\frac{\beta_t}{\sqrt{1-\bar{\alpha}_t}}\bm{\epsilon}_{\bm{\theta}}(\bm{x},\bm{y}^{(t)},G,t)\right), 
\end{align}
where $\bar{\alpha}_t$ is $\prod_{i=1}^t \alpha_i$. Here, parameterization of the residual function  $\epsilon_{\bm{\theta}}(\bm{x},\bm{y}^{(t)},G,t)$ enables residual-matching training objective \citep{ho2020denoising}, which is further simplification of \Cref{eq:ddpm_loss}. Specifically, we parameterize $\epsilon_{\bm{\theta}}(\bm{x},\bm{y}^{(t)},G,t)$ using a $L$-layer GNN as follows:
\begin{align*}
&\bm{\epsilon}_{\bm{\theta}}(\bm{x},\bm{y}^{(t)},G,t)=g(h^{(L)})\\
&h^{(\ell)}_{i}=(\text{COMBINE}^{(\ell)}(h^{(\ell-1)}_{i},a^{(\ell)}_{i})+f(t))\|y^{(t)}_i,\\
&a^{(\ell)}_{i} = \text{AGGREGATE}^{(\ell)}(\{h^{(\ell-1)}_{j} | (i, j) \in \mathcal{E}\}),
\end{align*}
where $g(h^{(L)})$ is an MLP that estimates the residual using the final node representation. $\text{AGGREGATE}(\cdot)$ and $\text{COMBINE}(\cdot)$ functions are identical to the backbone GNN, and $\cdot\|\cdot$ indicates the concatenation. Here, $h_i^{0}$ is initialized by concatenating the node features and noisy label $x_i\|y^{(t)}_i$. The $f(\cdot)$ is a time embedding function that consists of a sinusoidal positional embedding function \citep{vaswani2017attention} and two-layer MLP. In this paper, we fix the dimension of sinusoidal positional embedding to 128.

\subsection{Detailed training objective} \label{appx:architecture_loss} In \Cref{subsec:method-inductive}, we define the training objective of DPM-GSP in terms of estimated average $\bm{\mu}_{\bm{\theta}}(\bm{x},\bm{y}^{(t)},G,t)$. Here, \Cref{eq:epsilon_pred} enables defining the further simplified objective as follows: 
\begin{align*}
\mathcal{L}=\sum^{T}_{t=1}\mathbb{E}_{\bm{\epsilon}\sim\mathcal{N}(\mathbf{0},\mathbf{I})}\left[\frac{\beta_t^2}{2\sigma^2_t\alpha_t(1-\bar{\alpha}_t)}\left\| \bm{\epsilon}-\bm{\epsilon}_{\bm{\theta}}(\bm{x},\sqrt{\bar{\alpha}_t}\bm{y}^{(0)}+\sqrt{1-\bar{\alpha}_t}\bm{\epsilon},G,t)\right\|^2_2\right]
\end{align*}
where the detailed derivation follows \citet{ho2020denoising}. An additional suggestion from \citet{ho2020denoising} is to set all weights of the mean squared error to one instead of $\frac{\beta_t^2}{2\sigma^2_t\alpha_t(1-\bar{\alpha}_t)}$. We employ this idea by introducing a hyper-parameter called ``unweighted mean squared error'', with a True value indicating that all weights of the mean square error are set to one.
