# Supplementary material for: Diffusion Probabilistic Models for Structured Node Classification
Source: arXiv:2302.10506 source file (2023-06-19)
Supplement: Supplementary file 2 [file expanding.tex]

\section{Expanding few-layer GNN capabilities}

We also show that DPM-GSP expands the few-layer GNN capabilities. To be specific, we demonstrate that our model can distinguish non-isomorphic nodes with isomorphic local-hop neighborhoods, overcoming the conventional few-layer GNNs. The insight is based on the inference procedure of DPM-GSP, which recursive update of node-wise prediction with past predictions of neighboring targets. This allows structured prediction with a range of dependencies proportional to the number of diffusion steps. The details are described in \Cref{appx:th2}.
