# Supplementary material for: Diffusion Probabilistic Models for Structured Node Classification
Source: arXiv:2302.10506 source file (2023-06-19)
Supplement: Supplementary file 3 [file mcg.tex]

\section{Manifold-constrained sampling}
\label{appx:msg}

To sample $\bm{y}_U$ from $p_{\bm{\theta}}(\bm{y}_U|\bm{y}_L)$, we introduce a manifold-constrained sampling method proposed by \citet{chung2022improving}. Here, the update rule of the reverse process for $t=0,\ldots,T-1$ is modified as follows:
\begin{align*}
&\bm{y}'^{(t)}=\frac{1}{\sqrt{\alpha_t}}\left(\bm{y}^{(t+1)}-\frac{\beta_{t+1}}{\sqrt{1-\bar{\alpha}_{t+1}}}\bm{\epsilon}_{\bm{\theta}}(\bm{x},\bm{y}^{(t+1)},G,t+1)\right)+\sigma_{t+1}\bm{z}, \quad \mathbf{z} \sim \mathcal{N}(\mathbf{z};\mathbf{0},\lambda^2\mathbf{I}), \\
&\bm{y}^{(t)}_U=\bar{\mathbf{P}}\left(\bm{y}'^{(t)}-\gamma\frac{\partial}{\partial \bm{y}^{(t+1)}}\left\|\bm{y}_L - \mathbf{P}\hat{\bm{y}}\right\|^2_2\right)\\
&\bm{y}^{(t)}_L=\sqrt{\bar{\alpha}_{t}}\bm{y}_L+\sqrt{1-\bar{\alpha}_{t}}\mathbf{z},\quad\mathbf{z} \sim \mathcal{N}(\mathbf{z};\mathbf{0},\lambda^2 \mathbf{I}).
\end{align*}
The first equation is a temporal reverse diffusion step before applying the manifold-constrained samplings. The second equation applies the manifold-constrained gradient $\gamma\frac{\partial}{\partial \bm{y}^{(t+1)}}\left\|\bm{y}_L - \mathbf{P}\hat{\bm{y}}\right\|^2_2$, where $\mathbf{P}$ and $\bar{\mathbf{P}}$ is a masking matrix that selects the labeled nodes and unlabeled nodes, respectively. Here, $\hat{\bm{y}}$ is $\left(\bm{y}^{(t+1)}-\frac{1-{\bar{\alpha}_{t+1}}}{\sqrt{1-\bar{\alpha}_{t+1}}}\bm{\epsilon}_{\bm{\theta}}(\bm{x},\bm{y}^{(t+1)},G,t+1)\right)/\sqrt{\bar{\alpha}_{t+1}}$, and $\gamma$ is a hyper-parameter. Following \citet{chung2022improving}, we set $\gamma$ to $1/\left\|\bm{y}_L - \mathbf{P}\hat{\bm{y}}\right\|^2_2$. The third equation is a consistency step. Additionally, we introduce a parameter $\lambda$ to control the randomness; when we set $\lambda$ to zero, the modified reverse step becomes deterministic. We describe the detailed sampling algorithm in \Cref{alg:manifold_sampling}.

\begin{algorithm}[ht!] 
   \caption{Manifold-constrained sampling}\label{alg:manifold_sampling}
\begin{algorithmic}[1]
   \STATE \textbf{Input:} Graph $G$, node attributes $\bm{x}$, labels $\bm{y}_L$, and temperature of randomness $\lambda^2$.
   \STATE Get $\bm{y}^{(T)}\sim\mathcal{N}(\bm{y}^{(T)};\mathbf{0},\lambda^2\mathbf{I})$ \COMMENT{Initial sampling}
   \FOR{$t=T-1,\ldots,0$}
   \STATE Get $\bm{z}\sim\mathcal{N}(\bm{z};\mathbf{0},\lambda^2\mathbf{I})$
   \STATE $\bm{y}'^{(t)} \leftarrow \frac{1}{\sqrt{\alpha_t}}\left(\bm{y}^{(t+1)}-\frac{\beta_{t+1}}{\sqrt{1-\bar{\alpha}_{t+1}}}\bm{\epsilon}_{\bm{\theta}}(\bm{x},\bm{y}^{(t+1)},G,t+1)\right)+\sigma_{t+1}\bm{z}$ \COMMENT{Temporal reverse diffusion step}
   \STATE $\hat{\bm{y}} \leftarrow \left(\bm{y}^{(t+1)}-\frac{1-{\bar{\alpha}_{t+1}}}{\sqrt{1-\bar{\alpha}_{t+1}}}\bm{\epsilon}_{\bm{\theta}}(\bm{x},\bm{y}^{(t+1)},G,t+1)\right)/\sqrt{\bar{\alpha}_{t+1}}$
   \STATE $\bm{y}^{(t)}_U \leftarrow \bar{\mathbf{P}}\left(\bm{y}'^{(t)}-\gamma\frac{\partial}{\partial \bm{y}^{(t+1)}}\left\|\bm{y}_L - \mathbf{P}\hat{\bm{y}}\right\|^2_2\right)$ \COMMENT{Manifold-constrained gradient}
   \STATE Get $\bm{z}\sim\mathcal{N}(\bm{z};\mathbf{0},\lambda^2\mathbf{I})$
   \STATE $\bm{y}^{(t)}_L\leftarrow\sqrt{\bar{\alpha}_{t}}\bm{y}_L+\sqrt{1-\bar{\alpha}_{t}}\mathbf{z}$ \COMMENT{Consistency step}
   \STATE $\bm{y}^{(t)}\leftarrow \bm{y}^{(t)}_L\cup\bm{y}^{(t)}_U$
   \ENDFOR
   \STATE \textbf{return} $\bm{y}^{(0)}_U$
\end{algorithmic}
\end{algorithm}
