# Supplementary material for: Diffusion Probabilistic Models for Structured Node Classification
Source: arXiv:2302.10506 source file (2023-06-19)
Supplement: Supplementary file 4 [file reasoning.tex]

\section{Algorithmic reasoning}
\label{appx:reasoning}
